# Supplementary material for: Trends for isolated amino acids and dipeptides: Conformation, divalent ion binding, and remarkable similarity of binding to calcium and lead
Source: arXiv:1606.02151 source file (2016-09-14)

# Dipeptides

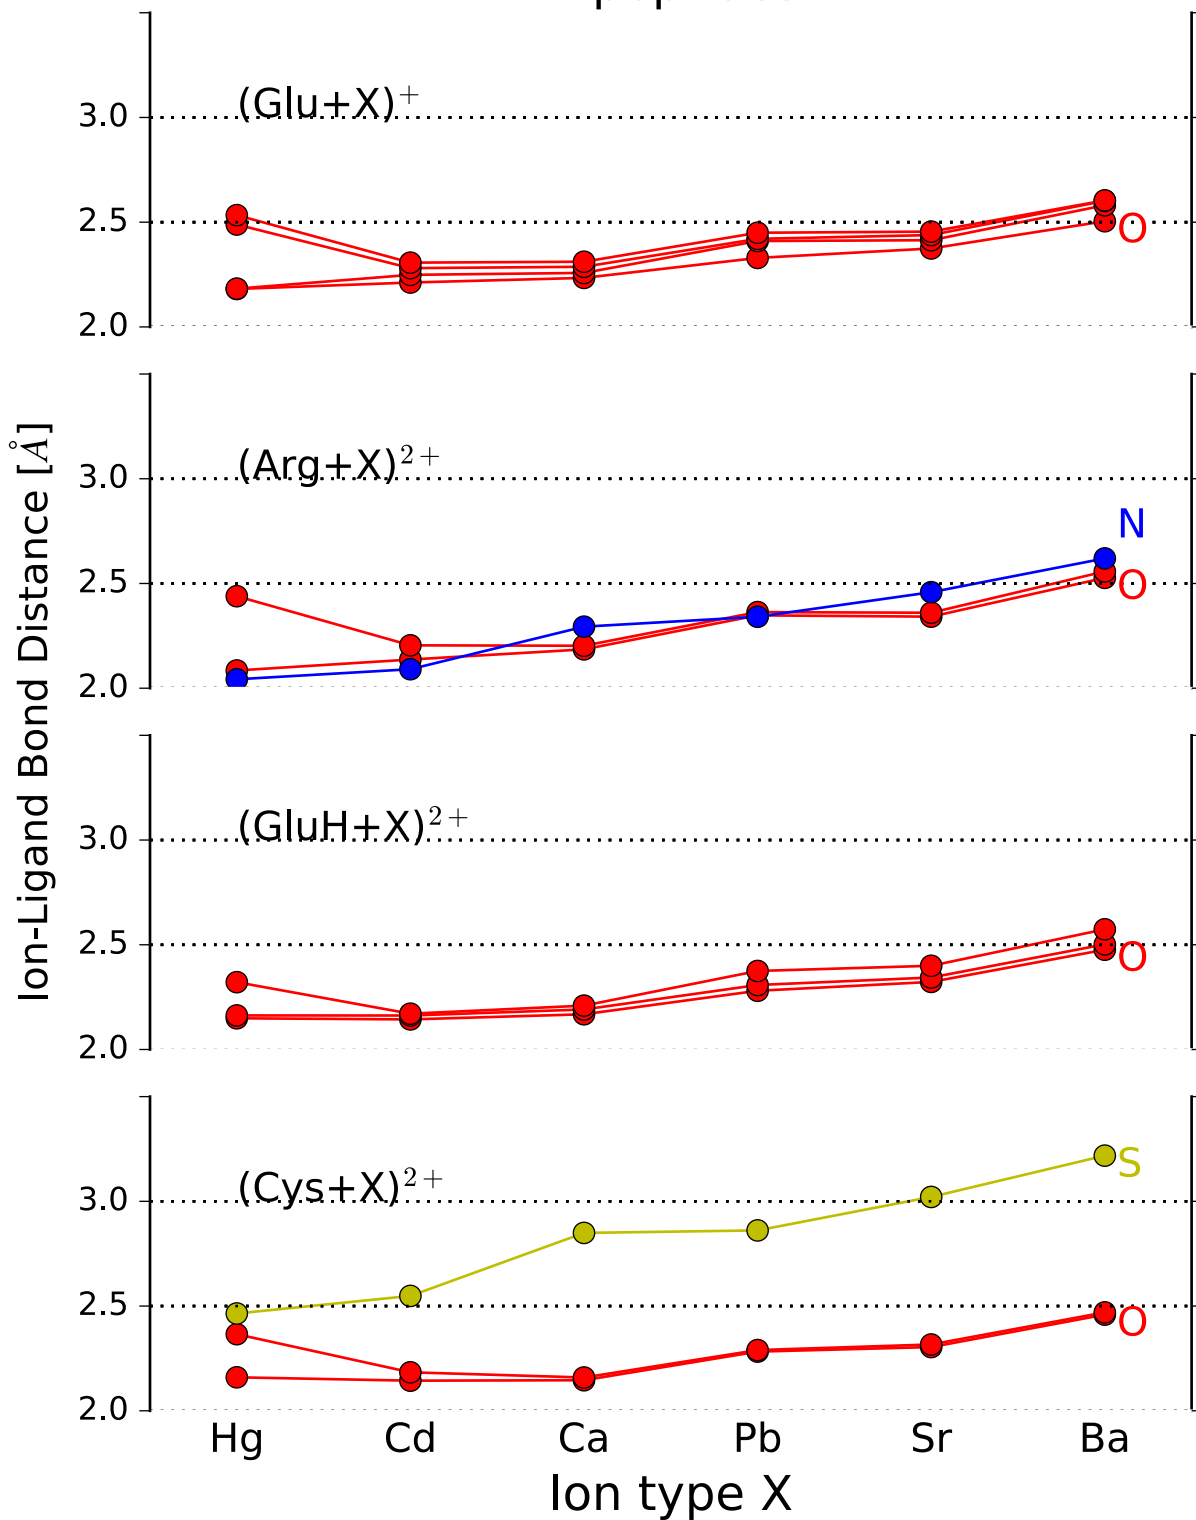

# Dipeptides

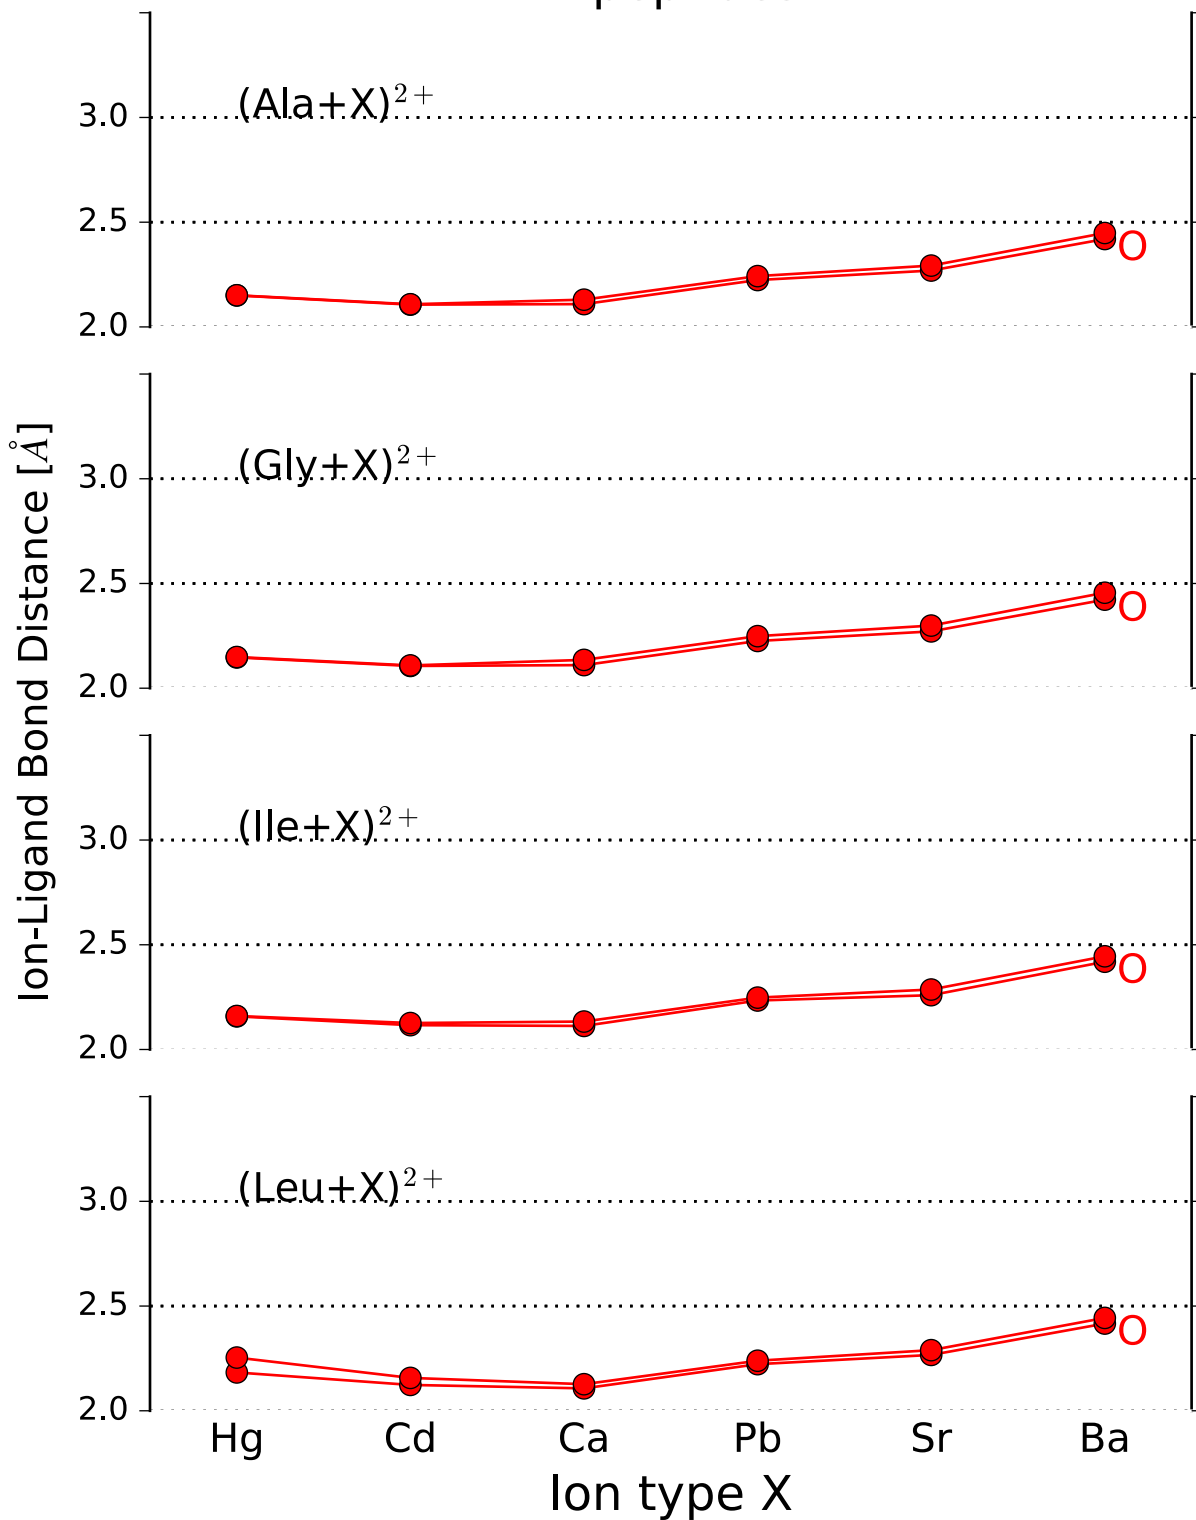

# Dipeptides

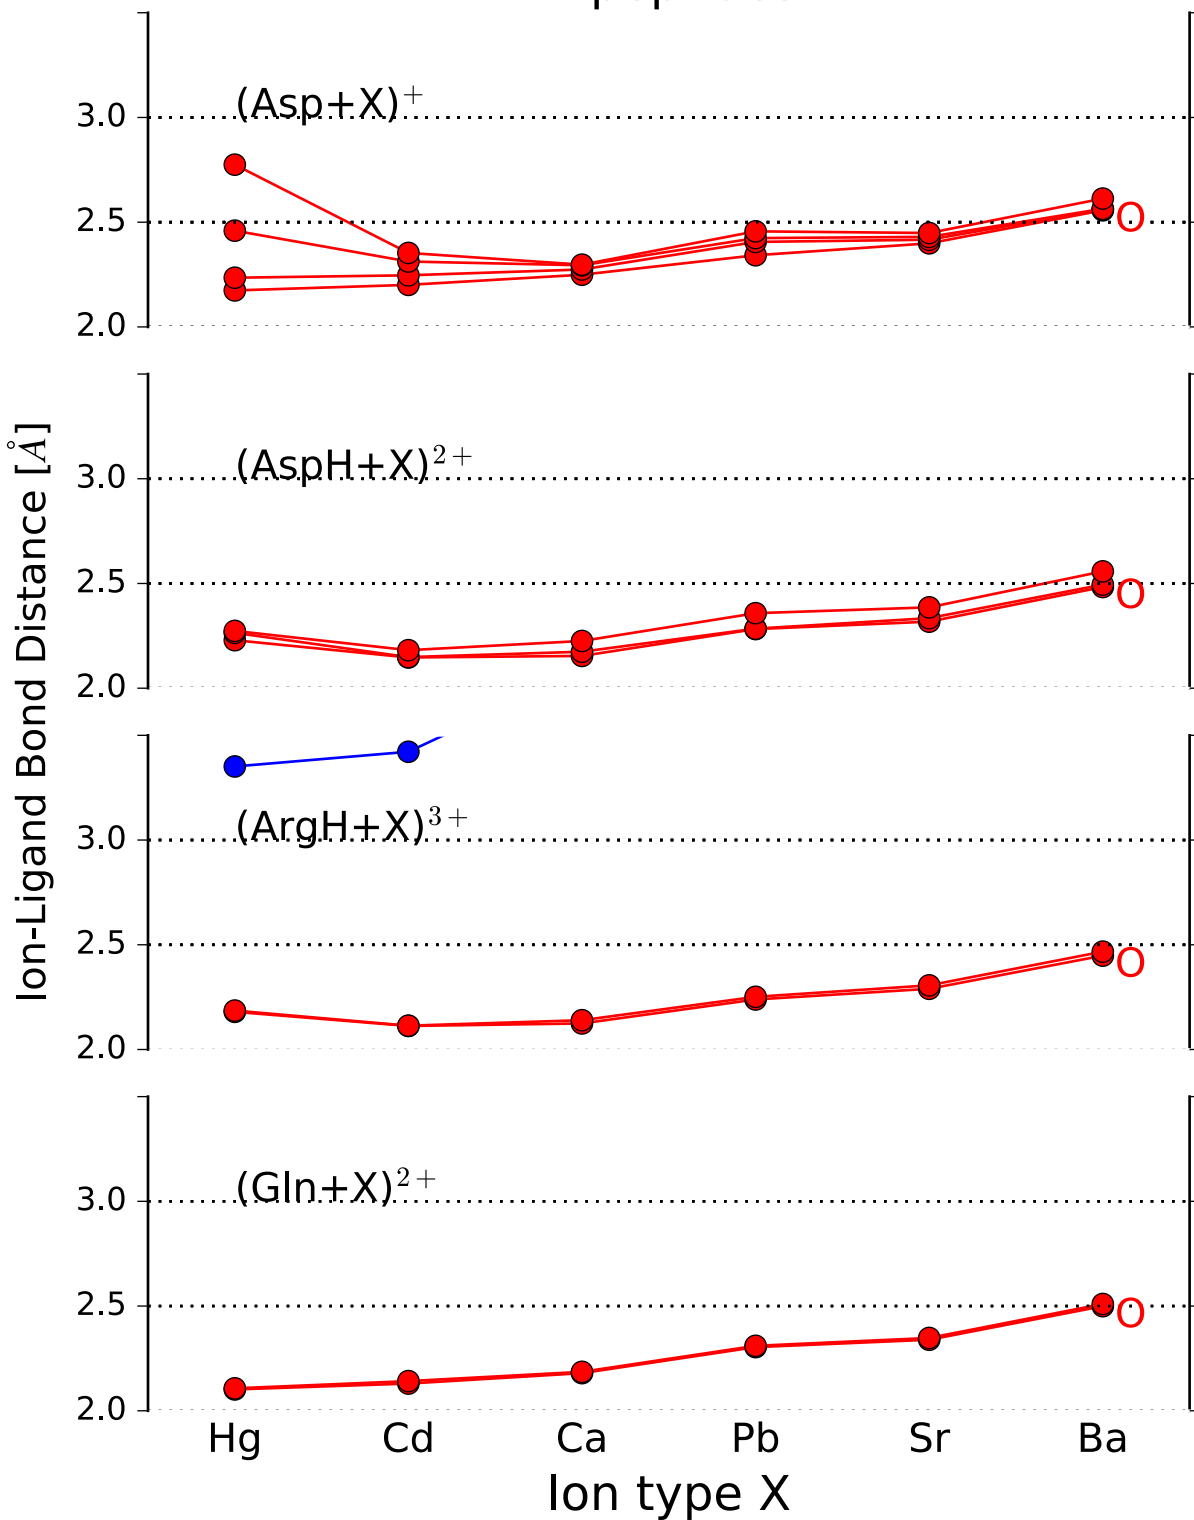

# Dipeptides

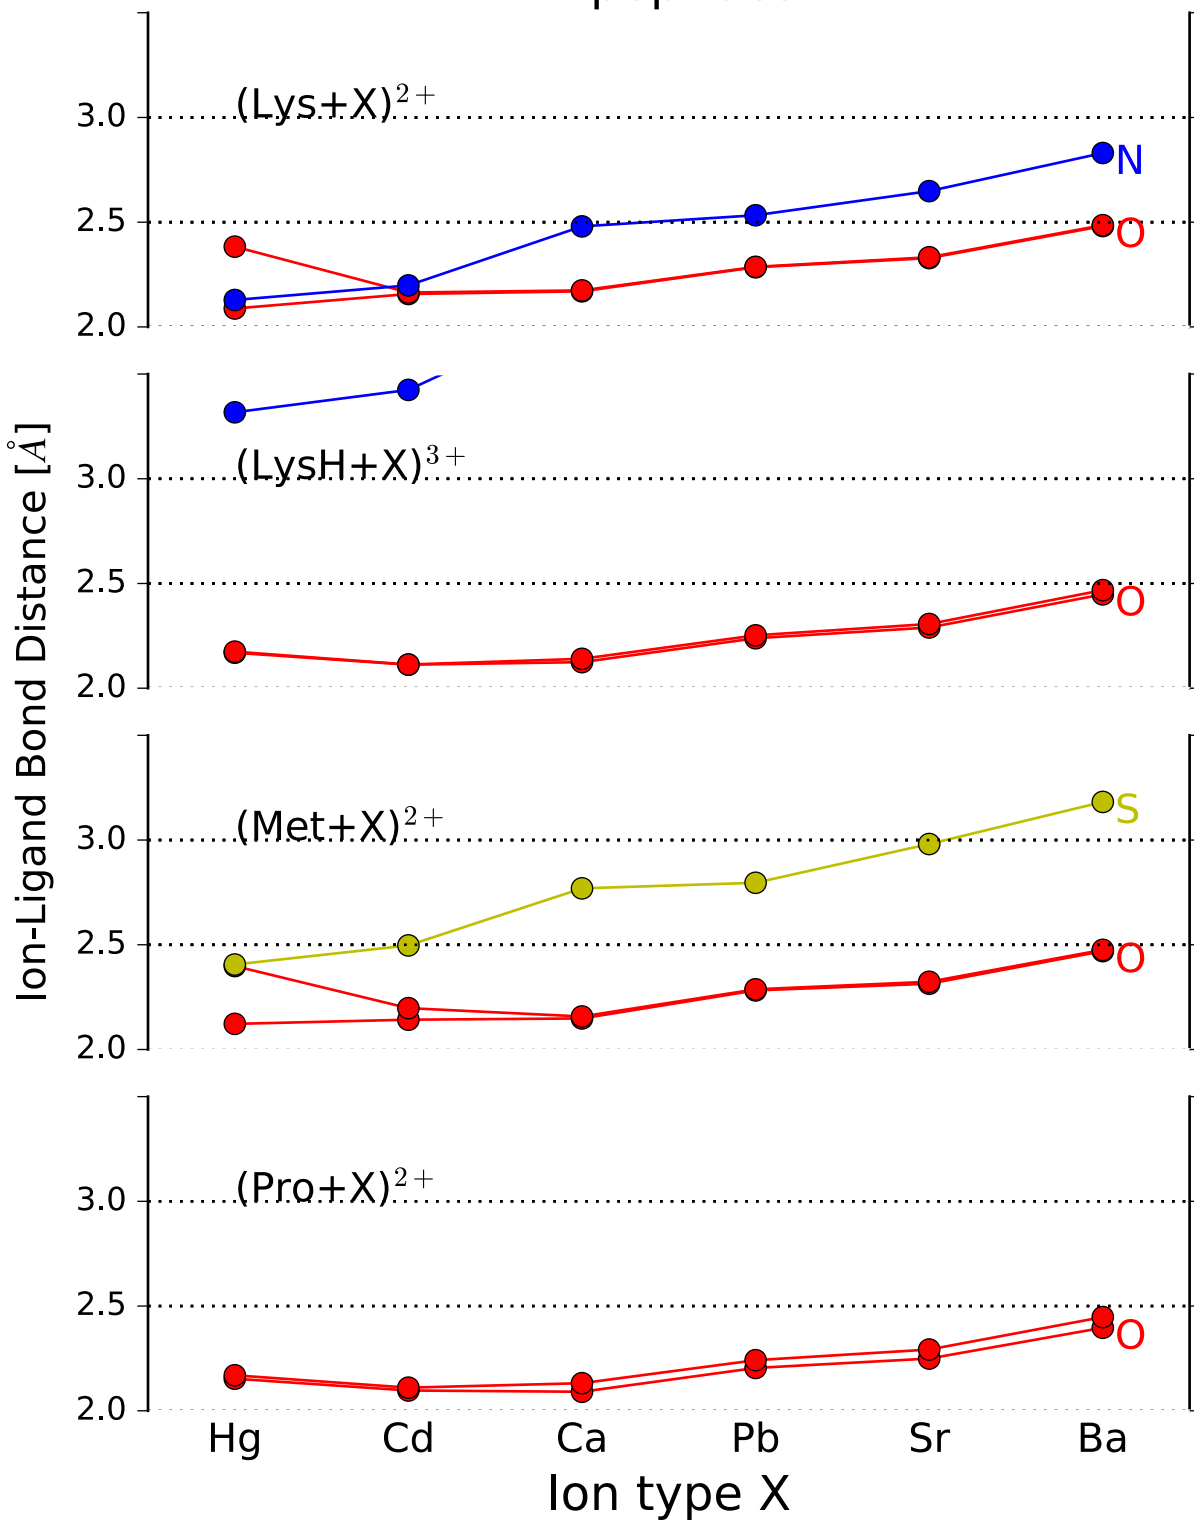

## Dipeptides

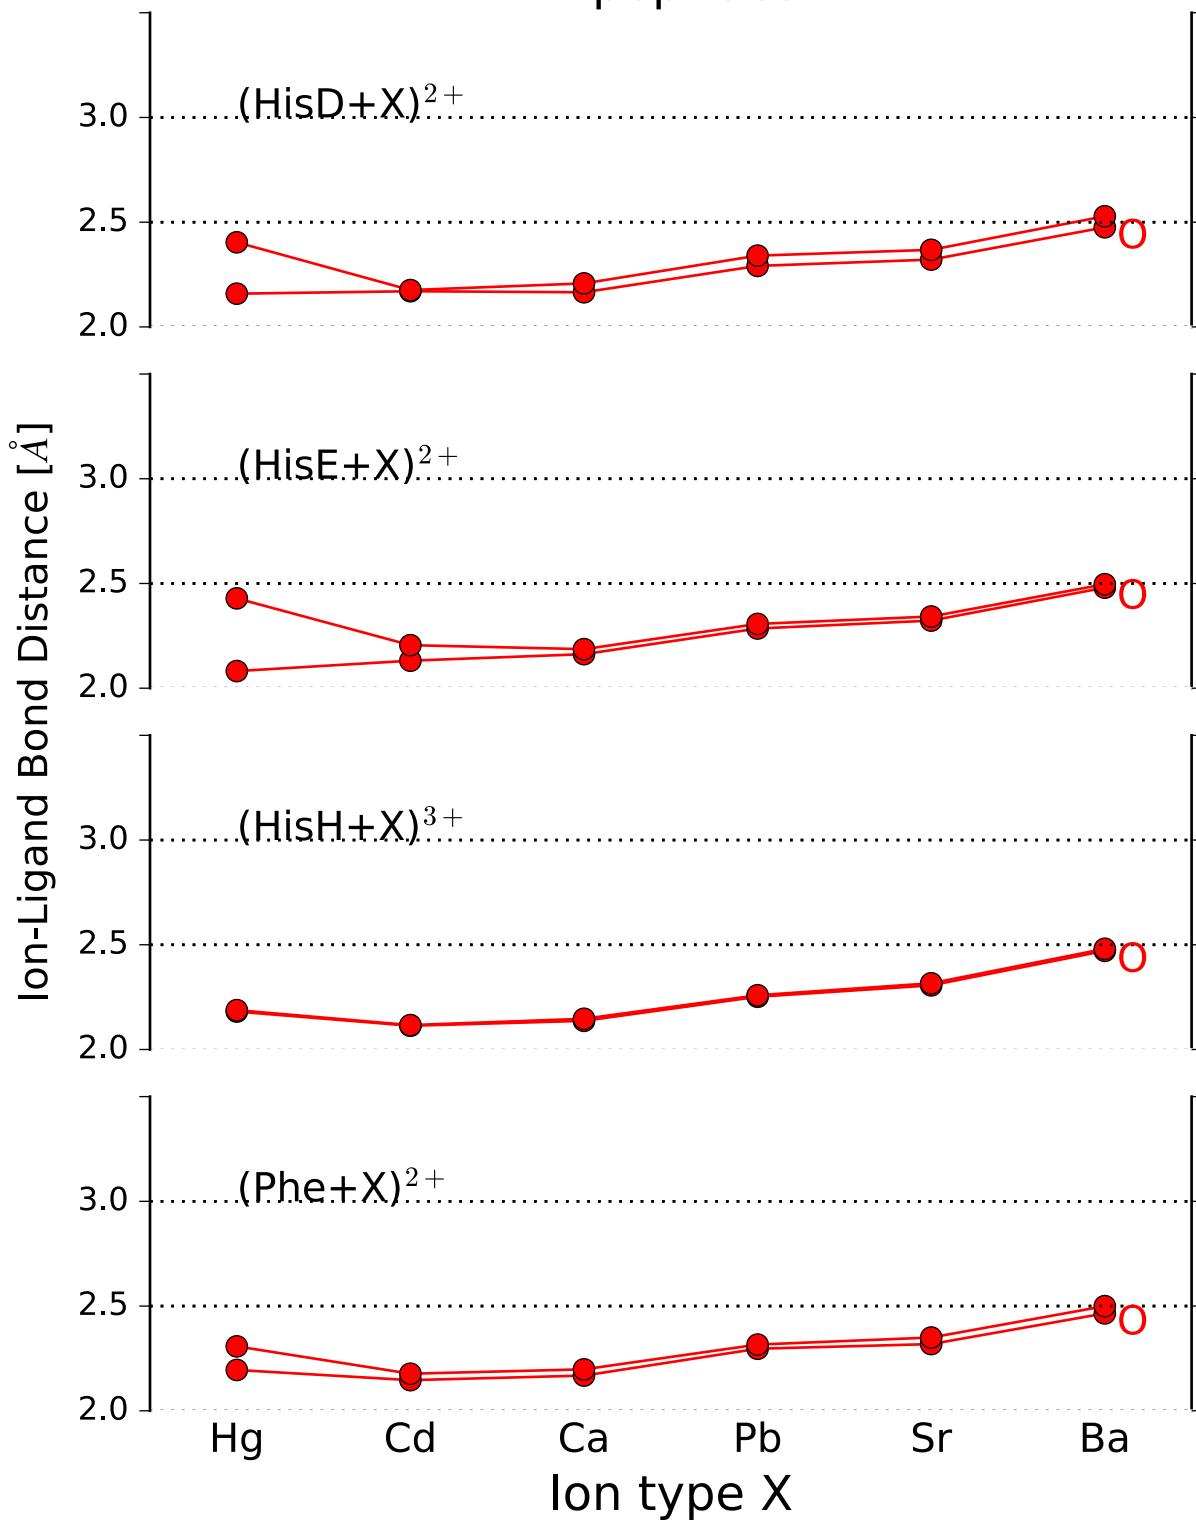

# Dipeptides

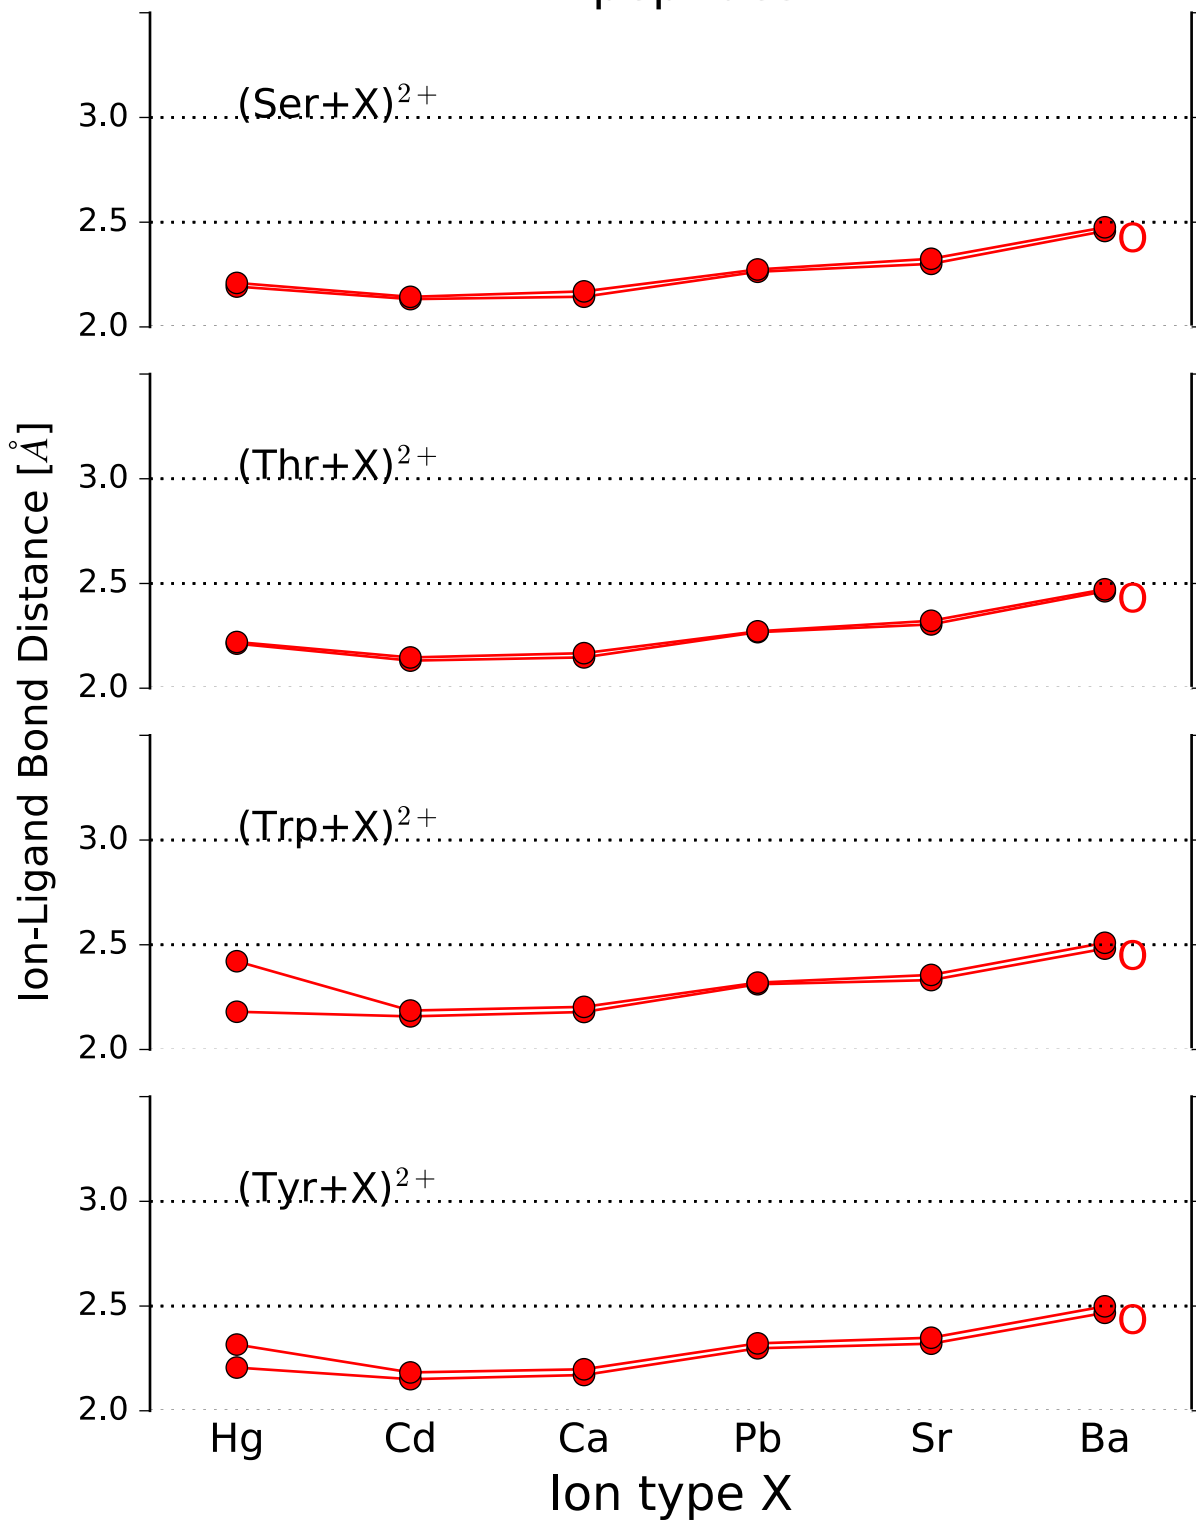

Supplement: Supplementary file 1 [file MRopo_Trends_r1_SuppInf.pdf]
